# Supplementary material for: Agentic Orchestration of HPC Applications in Cloud
Source: arXiv:2607.02925 source file (2026-07-03)
Supplement: Supplementary file 1 [file appendix.tex]

\newpage
\label{sec:appendix}
\section{Appendix}

\subsection{Applications}

% AMG
% BDAS
% CFDSCOPE
% CHATTERBUG
% CODESIGN KERNELS
% LAMMPS
% LAGHOS

\label{section:amg}
\smallskip
\noindent{\bf AMG2023} is provided via several builds across MPI variants, Ubuntu, and spack, and for CPU and GPU. We include AMG in our experiments, and ran problem 2 and used a problem size of 32x16x16 \cite{amg2023-github}. The \gls*{fom} is defined as: 

$FOM = \frac{nnz\_AP}{Setup Phase Time + 3*Solve Phase Time}$. 

In the above, nnz\_AP is the total number of non-zeros, and two timings for the setup and the solving phase \cite{amg2023-github}. We ran AMG2023 tests in a weak scaling configuration.

\label{section:bdas}
\smallskip
\noindent{\bf Big Data Analytics Benchmarks} (BDAS) \cite{schmidt2018definingbigdataanalytics} are a collection of data and \gls{ml} scientific models implemented in R that use \gls{mpi} for several well-known models (kmeans, svm, pca) that provide a holistic view of the capabilities of an environment. For our study we will run all three models with 250 rows, 50 columns for a problem size across scales. As was done in \cite{schmidt2018definingbigdataanalytics} we use the duration as the \gls{fom}.

% they seem to just use wall time https://arxiv.org/pdf/1811.02287

\label{section:cfdscope}
\smallskip
\noindent{\bf cfdSCOPE} (Computational Fluid Dynamics Scalability, Correctness, and Performance Estimator) is a set of mini-applications for computational fluid dynamics developed at TU Dresden that are intended for teaching \cite{cfdscope}. The benchmarks run on one node, and we worked with the main author to develop a variant that would strong scale across threads (11, 22, 44, 88) for each of 5 iterations for our study. The \gls{fom} is the time to complete one simulation at each size. 

\label{section:chatterbug}
\smallskip
\noindent{\bf chatterbug} 

% Running stencil3d on 5632 processors each with (1024, 1024, 1024) grid points with 4 variables
% Finished 100 iterations
% Time elapsed per iteration for grid size (1024,1024,1024) x 4 x 8: 0.612048 s

We used the stencil3d benchmark, a part the LLNL Chatterbug communication proxy suite, to emulate the communication patterns of scientific applications performing stencil computations on a 3D structured grid. We used a grid size of $1024^3$ and 100 iterations and measured the time to complete a halo exchange \cite{chatterbug}. This is a good library to evaluate general performance of scaled networking and \gls{mpi} libraries.

\label{section:e3sm-kernels}
\smallskip
\noindent{\bf e3sm kernels} 
are standalone, computationally intensive core routines extracted from Earth system model components \cite{Golaz2019-bu}. We will compile the Atmospheric kernels (the executable \emph{atm}) using spack \cite{gamblin2015spack} to run across scales.

% TODO what is the FoM? Duration?

\label{section:laghos}
\smallskip
\noindent{\bf Laghos} 
The LAGrangian High-Order Solver simulates the compression of gas using a moving frame~\cite{Dobrev2012-mm}. We used the major kernels total rate (megadofs $\times$ time steps/second) as our \gls*{fom}, and ran the app in a strong scaling configuration similar to the Vulcan example~\cite{laghos-github} with a \emph{cube\_311\_hex} mesh using partial assembly and a maximum of 400 steps. 

\label{section:lammps-reax}
\smallskip
\noindent{\bf LAMMPS} 
 is the Large-scale Atomic/Molecular Massively Parallel Simulator. It models the reaction of atoms and solves a matrix optimization problem. We are familiar with and thus used the \emph{ReaxFF} package, following a suggested practice \cite{lammps-reax} to calculate the millions of atom steps per second for our \gls*{fom}. A larger value is better, indicating a system can do more calculations per second. We chose a consistent problem size of 64x32x32 to run on GPU, and 64x64x32 for CPU for each of parameters x, y, and z, respectively. The GPU problem size was chosen to be smaller to fit on the GPUs on Google Cloud and \emph{B}. We ran LAMMPS in a strong scaling configuration.

\label{sec:ebpf-programs}
\subsection{\gls{ebpf} Programs}

\smallskip
\noindent{\it tcp}: We are interested to look at TCP-related system calls to get a glimpse of network activity, not just for our application, but other services running in Kubernetes that change with scale. Specifically, this program looks at data transfer sizes, call durations, and connection events. We again use tracepoints to attach to syscalls for sockets (connect, accept, close) and I/O calls (\emph{sendto}, \emph{recvfrom}, \emph{read} and \emph{write}), for each recording duration, return values, and bytes transferred. The data is sent to user-space via a ring buffer, where we again calculate RiverML statistics and counts for each. Since bytes transferred can fall within a large range, we group based on buckets of message sizes. From this program we can derive summary statistics for I/O operations broken down into buckets, including byte transfer and duration. If we see increased I/O call durations across scale, this could indicate the network stack taking longer to send and receive data, a possible result of the scaling. Higher latency or congestion that leads to longer syscall duration could mean increased round trip times or packet loss, contention within the TCP stack, or an application's slowness in receiving or processing data. 

% could it be buffer bloat? https://en.wikipedia.org/wiki/Bufferbloat
% breaking down operations into smaller ones and this overloads with too many syscalls?
% could it be there are too many added kubernetes tcp stuffs going on?
% if larger, could system take longer to fill large buffers?
% can network reliability decrease under high load?
% increase in transmissions because of data loss / errors
% are issues related to specific byte sizes?

\smallskip
\noindent{\it shared memory}: The shmem ``shared memory'' program traces calls for several operations (e.g., \emph{shmget} or \emph{shm\_open} or and \emph{shm\_unlink}), and calculates shared memory sizes to store in a BPF map keyed by the \gls{pid}. The command name is also saved. The maps are periodically read in user space, and at program completion, summary of operation counts and map sizes is produced, group by \gls{pid} and command. If we see increased shared memory usage as the application scales, this could suggest a higher demand for inter-process communication or other bottlenecks.

\label{sec:build-args}
\subsection{BuildKit Configurations}

\smallskip
\noindent{\bf Optimization Levels} 

We used BuildKit to generate containers across optimization levels \emph{O0} (no optimization), \emph{O1} (Basic optimizations) \emph{O2} (standard optimization), \emph{O3} (aggressive optimization), \emph{Ofast} (aggressive, non-compliant math), \emph{Os} (optimize for size), \emph{Og} (optimize for debugging) for each of arm64 and amd64 platforms.

\smallskip
\noindent{\bf Micro-architectures} 

For amd64 we built native, x86-64-v2, x86-64-v3,
x86-64-v4 (generic and portable based on instruction set levels), sandybridge, ivybridge, haswell, broadwell, skylake, skylake-avx512, icelake-server, sapphirerapids (Intel-specific), and btver2, bdver4, znver1, znver2, znver3 (AMD-specific). For arm64 we built native, neoverse-n1, neoverse-v1, neoverse-n2, neoverse-v2, ampere1, a64fx, cortex-a72, cortex-a53, cortex-a57, cortex-a76, cortex-x1, and generic micro-architectures.
